# Supplementary material for: An Ensemble Information Filter: Learning and Encoding Sparse Structures in Ensemble Kalman Methods
Source: arXiv:2501.09016 source file (2026-09-07)
Supplement: Supplementary file 1 [file appendix-6.tex]

\section{Information criteria for precision estimation / non-asymptotic TIC}
\label{app:information-criteria}

Low-sample-size Lorenz-96. AIC fails here. We want something that works.

Filtering: true model known to be outside space being searched over. So TIC.

But TIC uses Sandwich estimator, which uses sample covariance for variance of score.
Perhaps we can use a better estimator for the variance of the score (bootstrapped or shrinked (automatically?)), which' improvement will propagate through to TIC.

Test on low-sample-size Lorenz-96.
