# Supplementary material for: An Ensemble Information Filter: Learning and Encoding Sparse Structures in Ensemble Kalman Methods
Source: arXiv:2501.09016 source file (2026-09-07)
Supplement: Supplementary file 2 [file appendix-kalman-gain-variations.tex]

\section{Variations on ensemble Kalman gain}
\label{app:kalman-gain-variations}

Cite Raanes presentation EnKF 23

\begin{align*}
\bm{K} &= \Sigma_{x} \bm{H}^\top \Sigma_{d}^{-1}\\
&= \Sigma_{x} E[\nabla_{\bm{x}} \bm{h}(\bm{x})] \Sigma_{d}^{-1} \text{ using expected gradient (Stein's lemma)} \\
&\approx \frac{1}{n-1}\bm{X}\bm{X}^\top (\bm{Y}\bm{X}^{+})^\top \Sigma_{d}^{-1}
\text{ LLS (noisy) on map } \bm{h}: \bm{x}\mapsto \bm{y} \text{ or } E[\bm{d}]\\  
&= \frac{1}{n-1}\bm{X}\bm{Y}^\top\Sigma_{d}^{-1} \\
&\approx \hat{\Sigma}_{x,y}(\bm{Y}\bm{Y}^\top + \Sigma_\epsilon)^{-1} \text{ EnKF and ES variation} \\
&\approx \hat{\Sigma}_{x,y} (\bm{D}\bm{D}^\top)^{+}\\
&\approx \bm{X}\bm{D}^\top (\bm{D}\bm{D}^\top)^{+}\\
&=\bm{X}\bm{D}^+
\text{ LLS on map } \bm{h}^{-1}: \bm{d}\mapsto \bm{x}\\
&\to E[\nabla_{\bm{d}} \bm{h}^{-1}(\bm{d})]
\text{ again from Stein's lemma}
\end{align*}

Possible to recognize because $\bm{X}^\top(\bm{X}\bm{X}^\top)^+=\bm{X}^+$ for Moore-Penrose pseudoinverse.
